# Supplementary material for: Weak Ferromagnetism and Time-Stable Remanence in Hematite: Effect of Shape, Size and Morphology
Source: arXiv:1811.05231 source file (2018-11-13)
Supplement: Supplementary file 1 [file SI.pdf]

# Supplementary Material for
# "Weak Ferromagnetism and Time-Stable Remanence in Hematite: Effect of Shape, Size and Morphology"

Namrata Pattnayak,[1] Arpan Bhattacharyya,[2] Shruti Chakravarty,[1] and Ashna Bajpai[1,3]

[1]*Department of Physics, Indian Institute of Science Education and Research, Dr. Homi Bhabha Road, Pune 411008, India*
[2]*Saha Institute of Nuclear Physics, 1/AF Bidhannagar, Kolkata, India*
[3]*Center for Energy Science, Indian Institute of Science Education and Research, Dr. Homi Bhabha Road, Pune 411008, India*
(Dated: November 13, 2018)

## I. TEXT S1: SYNTHESIS

Hematite samples of different sizes and morphology have been synthesized by the hydrothermal method. For the synthesis of big cuboids and nano plates, hydrothermal methods described in [1] and [2] has been followed. Other hematite samples including small cuboids, micro plates and porous hematite have been synthesized by some minor modification employed in the hydrothermal routes as described below.

### A. Synthesis of hematite cuboids

For the synthesis of **big cuboids** 1.10 g of $FeCl_3.6H_2O$ and 1.21 g of urea first dissolved in 40 ml of distilled water (DW) under sonication. After complete dissolution, 2.82 ml of formamide is added into the solution. The mixture is then stirred properly and transferred into a teflon lined stainless steel autoclave (Parr instrument) of 45 ml capacity. The reaction carried out for 12 hours at a temperature of 160 °C in a normal oven (Memmert oven, UF55 Plus). After natural cooling of the autoclave to ambient temperature, the precipitate is collected by centrifugation and washed extensively using DW and ethanol. The collected precipitate finally dried at 80 °C for 7 hours before any characterization.

For the synthesis of **small cuboids** a little modification to the above synthesis condition has been followed. Keeping all the synthesis parameters constant, instead of $FeCl_3.6H_2O$, 1.18 g of $Fe(NO_3)_3.9H_2O$ was used as Fe precursor source for the synthesis of small cuboids.

### B. Synthesis of hematite plates

For **micro plates**, first solution 'A' prepared by dissolving 0.55 g of $FeCl_3.6H_2O$ in 10 ml of absolute ethanol. Solution B is then prepared by dissolving 1 g of NaOH pallets in 20 ml of DW. Solution A and B finally mixed properly under sonication for approximately 15 mins. The homogeneous mixture is then transfered into a 45 ml capacity of teflon lined stainless steel autoclave and heated at a temperature of 160 °C for 10 hours in a normal oven. The precipitate collected after the completion of reaction washed repeatadely using DW and ethanol and then dried at 80 °C for 7 hours before any characterization.

For the typical synthesis of **nano plates**, 0.55 g of $FeCl_3.6H_2O$ is first dissolved in 20 ml of ethanol containing trace addition ($\sim$ 1.4 ml) of DW. 1.6 g of Sodium acetate (NaOAc) then added into the solution. The mixture stirred approximately of about 20-30 mins for complete dissolution of NaOAc. The homogeneous mixture finally transfered into a 45 ml capacity of teflon lined stainless steel autoclave and the reaction carried out at a temperature of 180 °C for 12 hours in a normal oven. The precipitate collected after the completion of reaction washed repeatadely using DW and ethanol and then dried at 80 °C for 7 hours before characterization.

### C. Synthesis of Porous hematite

For the synthesis of **Porous** hematite first a 8 ml solution is prepared by dissolving 0.35 g of NaOH pallets in 8 ml DW. In the next step a separate 8 ml solution is prepared by dissolving 2.2 g of $FeCl_3.6H_2O$ in 8 ml of DW. Both the solution of volume ratio 1:1 then mixed properly under sonication and finally transferred into a teflon lined stainless steel autoclave of 45 ml capacity. The reaction carried out for 12 hours at a temperature of 160 °C. The precipitate formed after the completion of

reaction is collected by centrifugation followed by washing extensively using DW and ethanol. The collected precipate finally dried at 80 °C for 7 hours before all characterization.

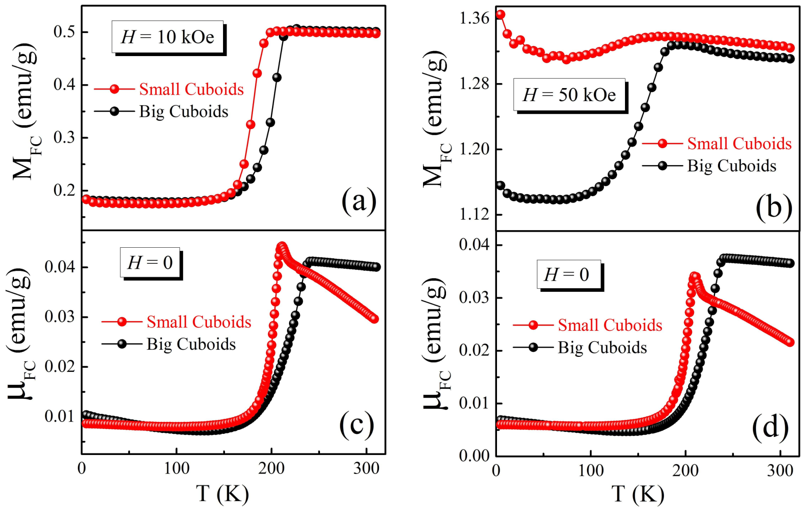


FIG. S1. $M_{FC}$ vs $T$ for big cuboids (black dots) and small cuboids (red dots) obtained at different magnetic fields of **(a)** $H$ = 10 kOe, **(b)** $H$ = 50 kOe. **(c)** and **(d)** compares the corresponding $\mu_{FC}$ vs $T$ data.

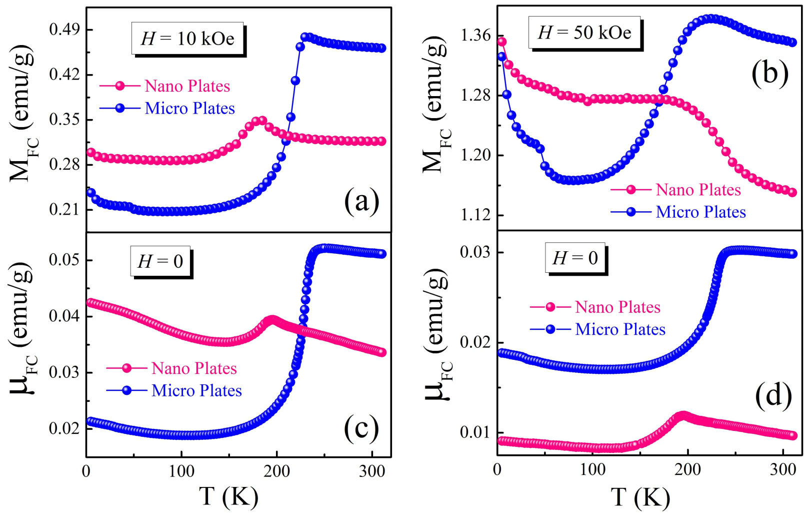


FIG. S2. $M_{FC}$ vs $T$ for micro plates (blue dots) and nano plates (pink dots) obtained at different magnetic fields of **(a)** $H$ = 10 kOe, **(b)** $H$ = 50 kOe. **(c)** and **(d)** compares the corresponding $\mu_{FC}$ vs $T$ data.

## II. TEXT S2: AFM EXCHANGE PATHWAY, BOND ANGLES AND LENGTHS

In Fig. S3 (a) the hexagonal unit cell of hematite is presented. The blue and orange balls represent the Fe atoms corresponding to the up and down spins. The superexchange pathways communicated between two different Fe atoms (between the blue and orange balls) via the intervening oxygen atom is marked by the red curves. The bond angle corresponding to the different

exchange pathways are labelled in the figure. Out of three different types of Fe-O-Fe bond angles and lengths, the temperature variation of two major Fe- O-Fe bond angles and the corresponding Fe-Fe bond lengths governing the basic AFM interaction in big cuboids and porous hematite samples is presented in Fig. S3 (b)-(e).

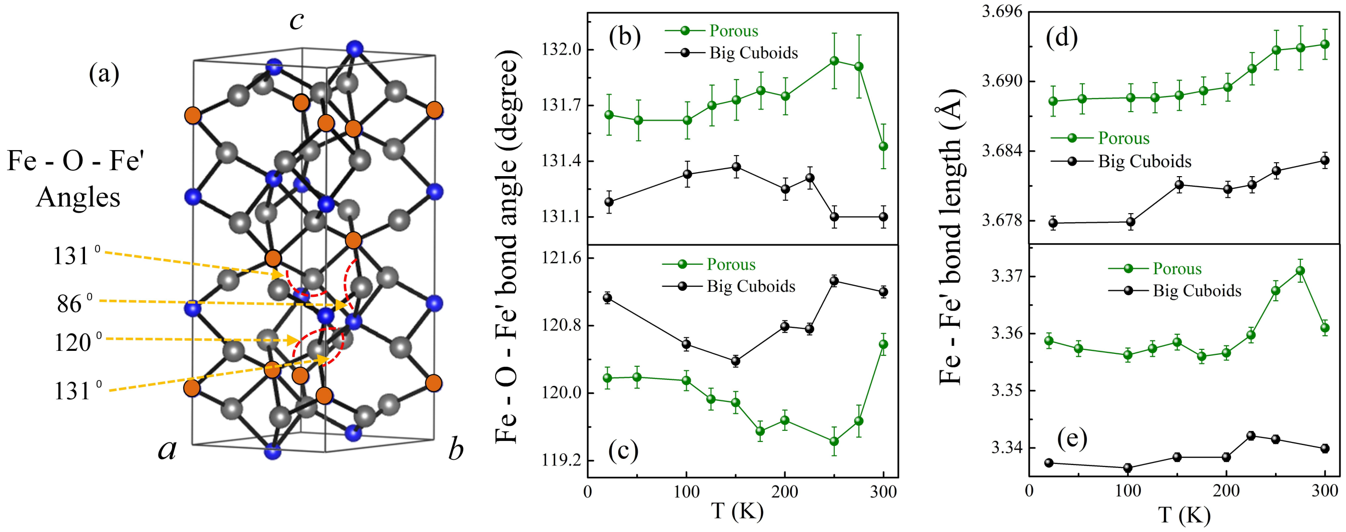


FIG. S3. **(a)** The hexagonal unit cell of hematite shown with the blue and orange balls representing the Fe atoms corresponding to up and down spins. The four different super exchange pathways and the corresponding bond angles are marked by the red curves. The temperature variation of bond angles **(b, c)** and bond lengths **(d, e)** governing the major superexchange pathways in big cuboids (black dots) and porous (green dots) hematite respectively.

[1] X. Liu, J. Zhang, S. Wu, D. Yang, P. Liu, H. Zhang, S. Wang, X. Yao, G. Zhu, and H. Zhao, RSC Adv. **2**, 6178 (2012).
[2] L. Chen, X. Yang, J. Chen, J. Liu, H. Wu, H. Zhan, C. Liang, and M. Wu, Inorganic Chemistry **49**, 8411 (2010).
